# Supplementary material for: Joint Expansion Planning of Power and Water Distribution Networks
Source: arXiv:2312.10224 source file (2023-12-15)
Supplement: Supplementary file 1 [file supporting_info.tex]

% **************************************
% Introduction *************************
% **************************************

% Water-energy nexus \cite{oikonomou2018optimal}
% \begin{itemize}
%     \item Quantification of dependence?
%     \begin{itemize}
%         \item  3-4 \% of electricity usage is for water infrastructure networks
%         \item Drinking and wastewater are the largest energy consumers of municipality government
%         \item California usage
%     \end{itemize}
%     \item Areas of interdependence
%     \begin{itemize}
%         \item Power on water: mining, fuel production, hydropower, power plant cooling
%         \item Water on power: pumping, distribution, waster water treatment
%     \end{itemize}
%     \item Intention and Practice
%     \begin{itemize}
%         \item They are designed to operate as uncoupled systems. However, they are interdependent
%     \end{itemize}
%     \item Consequences
%     \begin{itemize}
%         \item Vulnerability to cascading effects
%     \end{itemize}
%     \item Research questions
%     \begin{itemize}
%         \item Their behaviors to different types of disasters is different: hurricane effects on underground pipes vs overground power lines
%         \item {\color{blue}Q: Given that their operation is combined, can we take advantage of their dependence in improving the resilience of the joint networks and reducing the cost of expansion to meet the growing population's needs?
%     \end{itemize}
% \end{itemize}

% Their behaviors and vulnerability to different types of disasters is different. For example, underground pipes won't be impacted the same way as overground electric power lines. Even though water tanks are above ground, their number is far less in the overall network. Furthermore, recent tanks are designed to withstand wind speed of 150 mph. However, despite this enhanced resilience, water access is limited during disasters due to their dependency on power networks. Pump outages directly lead to an inability to circulate water across WDN. The dependency goes both ways: the amount of water storage reservoirs in rivers affects the ability to generate power.
% Networks are interwined. 

% However, their operation and expansion planning are separated. Combining this planning is expected to be beneficial, but there is a lack of quantification to realize its benefits. 
% This paper aims to address this gap by developing models to facilitate the expansion planning of power and water distribution networks and demonstrating the benefits of joint expansion planning.
